# Supplementary material for: Bayesian Model Calibration for Extrapolative Prediction via Gibbs Posteriors
Source: arXiv:1909.05428 source file (2019-09-12)
Supplement: Supplementary file 1 [file Appendix_Weight.tex]

Outside of calibration applications, there are many other suggestions for approaches to weight selection \citep{holmes2017assigning,miller2015robust,grunwald2017inconsistency,jiang2008gibbs,holmes2017assigning,
syring2017calibrating,lyddon2017generalized}. 
Cross-validation is commonly
used to select $w$ in power likelihood models from the machine
learning literature, deemed Gibbs posteriors and PAC Bayes methods
\citep{jiang2008gibbs}.  \cite{miller2015robust} refer to $w$ as the
``coarsening'' rate and select $w$ by conditioning on the event that
the empirical distribution of the observed data is close to the
model-based distribution, measuring closeness using relative entropy
(Kullback-Leibler divergence). They choose the learning rate based on
the tolerable difference in relative entropy, which is difficult to
interpret and tune.  Their approach provides a nice connection between
ABC and power-likelihood models.  \cite{grunwald2017inconsistency}
refer to $w$ as the learning rate and select $w$ based on the
predictive ability of the model, minimizing the ``posterior-expected
posterior-randomized log-loss function'', which is the expected loss
under the power-likelihood model if we actually sample from this
posterior.  This approach selects $w$ based on the predictive ability
of the model, choosing $w$ to minimize expected loss in a prequential
fashion.  The authors note that cross validation did perform similarly
toward the end of the article.  %Specifically, the power is selected to
%achieve a nominal frequentist coverage rate \sw{(of the predictive
 % intervals, if I recall\ldots)}, where the coverage is approximated
%using the bootstrap.  
\cite{holmes2017assigning} suggest choosing $w$
based on a relative change in Fisher information from prior to
posterior between two hypothetical experiments: one where the
parametric model is correct and another where the parametric model is
misspecified.

In similar bootstrap-based approaches, \cite{syring2017calibrating}
use frequentist coverage based on bootstrap resampling to select the
learning rate.  \cite{lyddon2017generalized} suggest choosing $w$ by
matching inferences under the distributions \eqref{eq:gibbs-posterior}
and \eqref{eq:bootstrap-model}.  Specifically, $w$ is selected to
match the Fisher information for the pseudo-posterior distribution of
$\theta$ from the Gibbs posterior \eqref{eq:gibbs-posterior} and the
bootstrapped distribution of $\theta (F)$ under
\eqref{eq:bootstrap-model}.  \cite{lyddon2017generalized} match the
trace of the information matrix between the two models, relying on
asymptotic results about the posterior distribution of $\theta$ under
the power likelihood and bootstrapped models.  They demonstrate that,
if \eqref{eq:bootstrap-model} is implemented under exchangeability
using a Bayesian bootstrap procedure, then both the power likelihood
\eqref{eq:gibbs-posterior} and Bayesian bootstrap posterior distributions for
$\theta$ asymptotically converge to a normal distribution.  Properties
of the asymptotic sampling distributions are used to select $w$.

%%% Local Variables:
%%% mode: latex
%%% TeX-master: "../Draft"
%%% End:
